# Supplementary material for: Charge pumps, boundary modes, and the necessity of unnecessary criticality
Source: arXiv:2408.15351 source file (2026-01-02)
Supplement: Supplementary file 2 [file SupMatSSBPhaseDiagram.tex]

%auto-ignore
\documentclass{standalone}
\usepackage{tikz, mathtools}
\usetikzlibrary{external}
\usetikzlibrary{decorations.pathmorphing}
\tikzset{snake it/.style={decorate,decoration={snake,segment length=2pt,amplitude=1pt}}}
\begin{document}
     \begin{tikzpicture}[scale=1.5]
		\draw[thick,->] (-0.35,-0.1) -- ++(4.5,0.0) node[align=right,below] {$J_U$};
		\draw[thick,->] (-0.35,-0.1) -- ++(0.0,3.) node[align=left,above] {$\delta$};
		\fill[blue,opacity=0.05] (-0.25,0.) rectangle ++(4.3,2.8);
%             \filldraw[red,opacity=0.1] (0.8,1.4) to[out=80,in=110] (3.9-0.8,1.4) to[out=-110,in=-80] (0.8,1.4);
    %      \fill[blue,opacity=0.1] (3.8/2-1.4,2.8) to[out=-90,in = 120] (3.8/2-1.,2.9/2) to[out=64,in=180-64] (3.8/2+1.,2.9/2) to[out=180-120,in=-90]  (3.8/2+1.4,2.8) --cycle;
    
            \fill[blue,opacity=0.1] (0.9,2.8) to[out=-90,in=120] (1.1,1.75) to[out=27,in=180-27] (3.8-1.1,1.75) to[in=-90,out=60] (3.8-0.9,2.8)--cycle;
            
            \draw[dashed] (0.9,2.8) to[out=-90,in=120] (1.1,1.75);
            \draw[dashed] (3.8-0.9,2.8) to[out=-90,in=60] (3.8-1.1,1.75);
            \draw[red] (3.8/2,2.9/2) ellipse (1.cm and .5cm);
            \fill[red,opacity=0.1] (3.8/2,2.9/2) ellipse (1.cm and .5cm);
            
             \draw[dotted] (0.1,2.8) to[out=-90,in=140] (0.6,1.8);
            \draw[dotted] (0.1,0) to[out=90,in=-140] (0.6,2.9-1.8);

            \draw[dotted] (3.8-0.1,2.8) to[out=-90,in=40] (3.8-0.6,1.8);
            \draw[dotted] (3.8-0.1,0) to[out=90,in=-40] (3.8-0.6,2.9-1.8);    
            \def\ya{1.15};
              \def\yb{1.3};
           \foreach   \x in {1.2,1.9} {\fill[rounded corners,gray,opacity=0.2] (\x,\ya) rectangle (\x+0.6,\ya+.6); 
              \node[] at(\x+0.18,\yb) {\scriptsize$\uparrow$};\node[] at(\x+0.4,\yb) {\scriptsize$\downarrow$};\node[] at(\x+0.18,\yb+0.27) {\scriptsize$\uparrow$};\node[] at(\x+0.4,\yb+0.27) {\scriptsize$\downarrow$};};

            \def\ya{2.25};
              \def\yb{2.38};
              \foreach   \x in {2.95} {\fill[rounded corners,gray,opacity=0.2] (\x,\ya) rectangle (\x+0.5,\ya+.5);\draw[blue, snake it]  (\x+0.15,\yb)--(\x+0.15,\yb+0.23); \draw[thick]  (\x+0.35,\yb+0.23)-- (\x+0.35,\yb)--(\x+0.55,\yb);\draw[thick]  (\x+0.35,\yb+0.23)--(\x+0.55,\yb+0.23);
              \shade[inner color=white, outer color = red] (\x+0.15,\yb) circle (0.06);\shade[inner color=white, outer color = red] (\x+0.35,\yb) circle (0.06);\shade[inner color=white, outer color = red] (\x+0.15,\yb+0.23) circle (0.06);\shade[inner color=white, outer color = red] (\x+0.35,\yb+0.23) circle (0.06);};

              \foreach   \x in {.3} {\fill[rounded corners,gray,opacity=0.2] (\x,\ya) rectangle (\x+0.5,\ya+.5);\draw[thick]  (\x+0.15,\yb)--(\x+0.15,\yb+0.23); \draw[thick]  (\x+0.35,\yb+0.23)--  (\x+0.35,\yb)--(\x+0.55,\yb);\draw[thick]  (\x+0.35,\yb+0.23)--(\x+0.55,\yb+0.23);
              \shade[inner color=white, outer color = red] (\x+0.15,\yb) circle (0.06);\shade[inner color=white, outer color = red] (\x+0.35,\yb) circle (0.06);\shade[inner color=white, outer color = red] (\x+0.15,\yb+0.23) circle (0.06);\shade[inner color=white, outer color = red] (\x+0.35,\yb+0.23) circle (0.06);};

               \foreach   \x in {1.6} {\fill[rounded corners,gray,opacity=0.2] (\x,\ya) rectangle (\x+0.5,\ya+.5);\draw[blue]  (\x+0.135,\yb+0.23)-- (\x+0.135,\yb);\draw[blue]  (\x+0.165,\yb+0.23)-- (\x+0.165,\yb); \draw[thick]  (\x+0.35,\yb+0.23)-- (\x+0.35,\yb)--(\x+0.55,\yb);\draw[thick]  (\x+0.35,\yb+0.23)--(\x+0.55,\yb+0.23);
              \shade[inner color=white, outer color = red] (\x+0.15,\yb) circle (0.06);\shade[inner color=white, outer color = red] (\x+0.35,\yb) circle (0.06);\shade[inner color=white, outer color = red] (\x+0.15,\yb+0.23) circle (0.06);\shade[inner color=white, outer color = red] (\x+0.35,\yb+0.23) circle (0.06);};
            
            \def\ya{1.15};
              \def\yb{1.28};
           \foreach   \x in {-.2} {\fill[rounded corners,gray,opacity=0.2] (\x,\ya) rectangle (\x+0.5,\ya+.5); \draw[thick]  (\x+0.15,\yb)--(\x+0.15,\yb+0.23);\draw[thick]  (\x+0.35,\yb)--(\x+0.35,\yb+0.23); 
              \shade[inner color=white, outer color = red] (\x+0.15,\yb) circle (0.06);\shade[inner color=white, outer color = red] (\x+0.35,\yb) circle (0.06);\shade[inner color=white, outer color = red] (\x+0.15,\yb+0.23) circle (0.06);\shade[inner color=white, outer color = red] (\x+0.35,\yb+0.23) circle (0.06);};

           \foreach   \x in {3.5} {\fill[rounded corners,gray,opacity=0.2] (\x,\ya) rectangle (\x+0.5,\ya+.5); \draw[blue, snake it]  (\x+0.15,\yb)--(\x+0.15,\yb+0.23);\draw[blue, snake it]  (\x+0.35,\yb)--(\x+0.35,\yb+0.23); 
              \shade[inner color=white, outer color = red] (\x+0.15,\yb) circle (0.06);\shade[inner color=white, outer color = red] (\x+0.35,\yb) circle (0.06);\shade[inner color=white, outer color = red] (\x+0.15,\yb+0.23) circle (0.06);\shade[inner color=white, outer color = red] (\x+0.35,\yb+0.23) circle (0.06);};              

              \def\ya{.05};
              \def\yb{.18};
              \foreach   \x in {1.65} {\fill[rounded corners,gray,opacity=0.2] (\x,\ya) rectangle (\x+0.5,\ya+.5); \draw[thick]  (\x+0.15,\yb) rectangle (\x+0.35,\yb+0.23);
              \shade[inner color=white, outer color = red] (\x+0.15,\yb) circle (0.06);\shade[inner color=white, outer color = red] (\x+0.35,\yb) circle (0.06);\shade[inner color=white, outer color = red] (\x+0.15,\yb+0.23) circle (0.06);\shade[inner color=white, outer color = red] (\x+0.35,\yb+0.23) circle (0.06);};
              
\node[] at(1.9,2.05) {\scriptsize DFSG};
\node[] at(1.9,3-2.15) {\scriptsize DFSG};
\node[rotate = 90] at(0.8,1.4) {\scriptsize SDSG};
\node[rotate = -90] at(3.8-0.8,1.4) {\scriptsize SDSG};
%\node[] at(1.9,1.9) {\scriptsize SSB};
\node[] at(1.9,-0.28) {0};
            \node[] at(-0.55,0.25) {-1};
            \node[] at(-0.55,1.4) {0};
            \node[] at(-0.55,2.7) {1};
\node[] at(1.9,3.0) {\scriptsize (a) $J_M\approx-5,~\Delta\approx 1.5$};
\node[] at (1.5,2.6) {\scriptsize T$_1$};
\node[] at (0.7,2.1) {\scriptsize T$_1$};
\node[] at (3.8-0.7,2.1) {\scriptsize T$_1$};
\node[] at (3.8-0.1,1.8) {\scriptsize T$_4$};
\node[] at (0.1,1.8) {\scriptsize T$_2$};
\node[] at (1.5,.2) {\scriptsize T$_1$};
		\end{tikzpicture}
  \begin{tikzpicture}[scale=1.5]
		\draw[thick,->] (-0.35,-0.1) -- ++(4.5,0.0) node[align=right,below] {$J_U$};
		\draw[thick,->] (-0.35,-0.1) -- ++(0.0,3.) node[align=left,above] {$\delta$};
		\fill[blue,opacity=0.05] (-0.25,0.) rectangle ++(4.3,2.8);
%             \filldraw[red,opacity=0.1] (0.8,1.4) to[out=80,in=110] (3.9-0.8,1.4) to[out=-110,in=-80] (0.8,1.4);
            \draw[red] (3.8/2,2.9/2) ellipse (1.cm and .5cm);
            \fill[red,opacity=0.1] (3.8/2,2.9/2) ellipse (1.cm and .5cm);
  
            \draw[dashed,blue] (3.8/2,2.75) -- (3.8/2,1.93);
    \draw[dotted] (.7,2.8) to[out=-90,in=140] (1.1,2);
    \draw[dotted] (.7,0) to[out=90,in=-140] (1.1,2.9-2);

       \draw[dotted] (3.8-.7,2.8) to[out=-90,in=40] (3.8-1.1,2);
    \draw[dotted] (3.8-.7,0) to[out=90,in=-40] (3.8-1.1,2.9-2);

            \def\ya{1.15};
              \def\yb{1.3};
           \foreach   \x in {1.2,1.9} {\fill[rounded corners,gray,opacity=0.2] (\x,\ya) rectangle (\x+0.6,\ya+.6); 
              \node[] at(\x+0.18,\yb) {\scriptsize$\uparrow$};\node[] at(\x+0.4,\yb) {\scriptsize$\downarrow$};\node[] at(\x+0.18,\yb+0.27) {\scriptsize$\downarrow$};\node[] at(\x+0.4,\yb+0.27) {\scriptsize$\uparrow$};};

            \def\ya{2.2};
              \def\yb{2.33};
              \foreach   \x in {2} {\fill[rounded corners,gray,opacity=0.2] (\x,\ya) rectangle (\x+0.5,\ya+.5);\draw[blue, snake it]  (\x+0.15,\yb)--(\x+0.15,\yb+0.23); \draw[thick]  (\x+0.35,\yb+0.23)-- (\x+0.35,\yb)--(\x+0.55,\yb);\draw[thick]  (\x+0.35,\yb+0.23)--(\x+0.55,\yb+0.23);
              \shade[inner color=white, outer color = red] (\x+0.15,\yb) circle (0.06);\shade[inner color=white, outer color = red] (\x+0.35,\yb) circle (0.06);\shade[inner color=white, outer color = red] (\x+0.15,\yb+0.23) circle (0.06);\shade[inner color=white, outer color = red] (\x+0.35,\yb+0.23) circle (0.06);};

              \foreach   \x in {1.28} {\fill[rounded corners,gray,opacity=0.2] (\x,\ya) rectangle (\x+0.5,\ya+.5);\draw[thick]  (\x+0.15,\yb)--(\x+0.15,\yb+0.23); \draw[thick]  (\x+0.35,\yb+0.23)--  (\x+0.35,\yb)--(\x+0.55,\yb);\draw[thick]  (\x+0.35,\yb+0.23)--(\x+0.55,\yb+0.23);
              \shade[inner color=white, outer color = red] (\x+0.15,\yb) circle (0.06);\shade[inner color=white, outer color = red] (\x+0.35,\yb) circle (0.06);\shade[inner color=white, outer color = red] (\x+0.15,\yb+0.23) circle (0.06);\shade[inner color=white, outer color = red] (\x+0.35,\yb+0.23) circle (0.06);};

            \def\ya{1.15};
              \def\yb{1.28};
           \foreach   \x in {-.2} {\fill[rounded corners,gray,opacity=0.2] (\x,\ya) rectangle (\x+0.5,\ya+.5); \draw[thick]  (\x+0.15,\yb)--(\x+0.15,\yb+0.23);\draw[thick]  (\x+0.35,\yb)--(\x+0.35,\yb+0.23); 
              \shade[inner color=white, outer color = red] (\x+0.15,\yb) circle (0.06);\shade[inner color=white, outer color = red] (\x+0.35,\yb) circle (0.06);\shade[inner color=white, outer color = red] (\x+0.15,\yb+0.23) circle (0.06);\shade[inner color=white, outer color = red] (\x+0.35,\yb+0.23) circle (0.06);};

           \foreach   \x in {3.5} {\fill[rounded corners,gray,opacity=0.2] (\x,\ya) rectangle (\x+0.5,\ya+.5); \draw[blue, snake it]  (\x+0.15,\yb)--(\x+0.15,\yb+0.23);\draw[blue, snake it]  (\x+0.35,\yb)--(\x+0.35,\yb+0.23); 
              \shade[inner color=white, outer color = red] (\x+0.15,\yb) circle (0.06);\shade[inner color=white, outer color = red] (\x+0.35,\yb) circle (0.06);\shade[inner color=white, outer color = red] (\x+0.15,\yb+0.23) circle (0.06);\shade[inner color=white, outer color = red] (\x+0.35,\yb+0.23) circle (0.06);};              

              \def\ya{.1};
              \def\yb{.23};
              \foreach   \x in {1.65} {\fill[rounded corners,gray,opacity=0.2] (\x,\ya) rectangle (\x+0.5,\ya+.5); \draw[thick]  (\x+0.15,\yb) rectangle (\x+0.35,\yb+0.23);
              \shade[inner color=white, outer color = red] (\x+0.15,\yb) circle (0.06);\shade[inner color=white, outer color = red] (\x+0.35,\yb) circle (0.06);\shade[inner color=white, outer color = red] (\x+0.15,\yb+0.23) circle (0.06);\shade[inner color=white, outer color = red] (\x+0.35,\yb+0.23) circle (0.06);};
              
\node[] at(1.9,2.05) {\scriptsize DFSG};
\node[] at(1.9,3-2.2) {\scriptsize DFSG};
\node[rotate = 90] at(0.8,1.4) {\scriptsize SDSG};
\node[rotate = -90] at(3.8-0.8,1.4) {\scriptsize SDSG};
%\node[] at(1.9,1.9) {\scriptsize SSB};
\node[] at(1.9,-0.28) {0};
            \node[] at(-0.55,0.25) {-1};
            \node[] at(-0.55,1.4) {0};
            \node[] at(-0.55,2.7) {1};
 
\node[] at (1.1,2.5) {\scriptsize T$_1$};
\node[] at (3.8-1.1,2.5) {\scriptsize T$_1$};
\node[] at (3.8-0.1,1.8) {\scriptsize T$_4$};
\node[] at (0.1,1.8) {\scriptsize T$_2$};
\node[] at (1.5,.2) {\scriptsize T$_1$};
\node[] at(1.9,3.0) {\scriptsize (b) $J_M \approx 5,~\Delta \approx 1.5$};
		\end{tikzpicture}
\end{document}
