# Supplementary material for: Charge pumps, boundary modes, and the necessity of unnecessary criticality
Source: arXiv:2408.15351 source file (2026-01-02)
Supplement: Supplementary file 3 [file SupMatUCPhasediagram.tex]

%auto-ignore
\documentclass{standalone}
\usepackage{tikz, mathtools}
\usetikzlibrary{external}
\usetikzlibrary{decorations.pathmorphing}
\tikzset{snake it/.style={decorate,decoration={snake,segment length=2pt,amplitude=1pt}}}
\begin{document}
\begin{tikzpicture}[scale = 1.5]
		\draw[thick,->] (-0.6,-0.1) -- ++(7.,0.0) node[align=right,below] {$J_U$};
		\draw[thick,->] (-0.6,-0.1) -- ++(0.0,3.) node[align=left,above] {$\delta$};
		\fill[blue,opacity=0.05] (-0.5,0.) rectangle ++(6.8,2.8);
 
    \draw[dotted] (6.,2.8) to[out=-90,in=20] (5,1.8);
    \draw[dotted] (6,0) to[out=90,in=-20] (5,2.8-1.8);

   \draw[dotted] (-0.2,2.8) to[out=-90,in=160] (0.8,1.8);
    \draw[dotted] (-0.2,0) to[out=90,in=-160] (0.8,2.8-1.8);
  
            \draw[thick] (2,1.4) -- (5.8-2,2.8-1.4);
            \fill[red] (2,1.4) circle (0.05);
            \fill[red] (5.8-2,2.8-1.4) circle (0.05);
            \fill[blue,opacity=0.1] (1.6,2.8) to[out=-90,in = 140] (2,1.4) -- (5.8-2,1.4) to[out=40,in=-90]  (5.8-1.6,2.8) -- cycle;
            \draw[dashed] (1.6,2.8) to[out=-90,in = 140] (2,1.4);
            \draw[dashed]  (5.8-1.6,2.8)to[in=40,out=-90]  (5.8-2,1.4);

            \fill[green,opacity=0.2,rounded corners] (2,1.4) to[bend left] (1.3,2) to[bend right] (1.3,0.8) to[bend left] (2,1.4);
            \draw[rounded corners] (2,1.4) to[bend left] (1.3,2) to[bend right] (1.3,0.8) to[bend left] (2,1.4);
            \fill[yellow,opacity=0.2,rounded corners] (5.8-2,1.4) to[bend right] (5.8-1.3,2)  to[bend left] (5.8-1.3,0.8) to[bend right] (5.8-2,1.4)  ;
            \draw[rounded corners] (5.8-2,1.4) to[bend right] (5.8-1.3,2)  to[bend left] (5.8-1.3,0.8) to[bend right] (5.8-2,1.4) ;
            \node[] at(1.42,1.4) {\scriptsize XY$_1^*$};
            \node[] at(4.41,1.4) {\scriptsize XY$_1$};
            \node[] at(2.9,1.52) {\scriptsize XY$_2$};

            \node[] at(2.2,2.5) {\scriptsize T$_1$};
            \node[] at(0.2,2.5) {\scriptsize T$_1$};
            \node[] at(5.6,2.5) {\scriptsize T$_1$};

            \node[] at(2.2,0.3) {\scriptsize T$_3$};

            \node[] at(0.0,1.8) {\scriptsize T$_2$};
            \node[] at(5.8,1.8) {\scriptsize T$_4$};

            \node[] at(2.9,-0.25) {0};
            \node[] at(-0.8,0.25) {-1};
            \node[] at(-0.8,1.4) {0};
            \node[] at(-0.8,2.7) {1};
              \node[] at(2.9,1) {\scriptsize $c=3/2$};
              \draw[->,thin] (2.4,1.05) -- (2.05,1.3);
              \draw[->,thin] (3.4,1.05) -- (3.75,1.3);
              
              \def\ya{.1};
              \def\yb{.23};
              \foreach   \x in {2.4,3.0} {\fill[rounded corners,gray,opacity=0.2] (\x,\ya) rectangle (\x+0.5,\ya+.5); \draw[thick]  (\x+0.15,\yb) rectangle(\x+0.35,\yb+0.23);
              \shade[inner color=white, outer color = red] (\x+0.15,\yb) circle (0.06);\shade[inner color=white, outer color = red] (\x+0.35,\yb) circle (0.06);\shade[inner color=white, outer color = red] (\x+0.15,\yb+0.23) circle (0.06);\shade[inner color=white, outer color = red] (\x+0.35,\yb+0.23) circle (0.06);};
              
              \def\ya{2.2};
              \def\yb{2.33};
              \foreach \x in {3.15} {\draw[thick]   (\x+0.45,\yb+0.23)--(\x+0.2,\yb+0.23)-- (\x+0.2,\yb)--(\x+0.45,\yb);}
              \foreach \x in {3.0} {\draw[thick]  (\x+0.15,\yb) rectangle (\x-0.25,\yb+0.23);}
              \foreach   \x in {2.4} {\draw[blue]  (\x+0.135,\yb+0.23)-- (\x+0.135,\yb);\draw[blue]  (\x+0.165,\yb+0.23)-- (\x+0.165,\yb);}
              \foreach   \x in {2.4,3.0} {\fill[rounded corners,gray,opacity=0.2] (\x,\ya) rectangle (\x+0.5,\ya+.5); 
              \shade[inner color=white, outer color = red] (\x+0.15,\yb) circle (0.06);\shade[inner color=white, outer color = red] (\x+0.35,\yb) circle (0.06);\shade[inner color=white, outer color = red] (\x+0.15,\yb+0.23) circle (0.06);\shade[inner color=white, outer color = red] (\x+0.35,\yb+0.23) circle (0.06);};

              \def\sh{-2.05};
              \foreach \x in {3.15+\sh} {\draw[thick] (\x+0.45,\yb+0.23)--(\x+0.2,\yb+0.23)-- (\x+0.2,\yb)--(\x+0.45,\yb);}
              \foreach \x in {3.0+\sh} {\draw[thick]  (\x+0.15,\yb) rectangle (\x-0.25,\yb+0.23);}
              \foreach   \x in {2.4+\sh} {\draw[thick]  (\x+0.15,\yb+0.23)-- (\x+0.15,\yb);}
              \foreach   \x in {2.4+\sh,3.0+\sh} {\fill[rounded corners,gray,opacity=0.2] (\x,\ya) rectangle (\x+0.5,\ya+.5); 
              \shade[inner color=white, outer color = red] (\x+0.15,\yb) circle (0.06);\shade[inner color=white, outer color = red] (\x+0.35,\yb) circle (0.06);\shade[inner color=white, outer color = red] (\x+0.15,\yb+0.23) circle (0.06);\shade[inner color=white, outer color = red] (\x+0.35,\yb+0.23) circle (0.06);};
            
            \def\sh{1.85};
              \foreach \x in {3.15+\sh} {\draw[thick] (\x+0.45,\yb+0.23)--(\x+0.2,\yb+0.23)-- (\x+0.2,\yb)--(\x+0.45,\yb);}
              \foreach \x in {3.0+\sh} {\draw[thick]  (\x+0.15,\yb) rectangle (\x-0.25,\yb+0.23);}
              \foreach   \x in {2.4+\sh} {\draw[blue, snake it]  (\x+0.15,\yb+0.23)-- (\x+0.15,\yb);}
              \foreach   \x in {2.4+\sh,3.0+\sh} {\fill[rounded corners,gray,opacity=0.2] (\x,\ya) rectangle (\x+0.5,\ya+.5); 
              \shade[inner color=white, outer color = red] (\x+0.15,\yb) circle (0.06);\shade[inner color=white, outer color = red] (\x+0.35,\yb) circle (0.06);\shade[inner color=white, outer color = red] (\x+0.15,\yb+0.23) circle (0.06);\shade[inner color=white, outer color = red] (\x+0.35,\yb+0.23) circle (0.06);};
              
              \def\sh{0.45};
            \def\ya{1.15};
              \def\yb{1.28};
           \foreach   \x in {4.75+\sh,5.3+\sh} {\fill[rounded corners,gray,opacity=0.2] (\x,\ya) rectangle (\x+0.5,\ya+.5); \draw[blue, snake it]  (\x+0.15,\yb)--(\x+0.15,\yb+0.23);\draw[blue, snake it]  (\x+0.35,\yb)--(\x+0.35,\yb+0.23); 
              \shade[inner color=white, outer color = red] (\x+0.15,\yb) circle (0.06);\shade[inner color=white, outer color = red] (\x+0.35,\yb) circle (0.06);\shade[inner color=white, outer color = red] (\x+0.15,\yb+0.23) circle (0.06);\shade[inner color=white, outer color = red] (\x+0.35,\yb+0.23) circle (0.06);}

           \def\sh{-0.45};
           \foreach   \x in {0.0+\sh,0.55+\sh} {\fill[rounded corners,gray,opacity=0.2] (\x,\ya) rectangle (\x+0.5,\ya+.5); \draw[thick]  (\x+0.15,\yb)--(\x+0.15,\yb+0.23);\draw[thick]  (\x+0.35,\yb)--(\x+0.35,\yb+0.23); 
              \shade[inner color=white, outer color = red] (\x+0.15,\yb) circle (0.06);\shade[inner color=white, outer color = red] (\x+0.35,\yb) circle (0.06);\shade[inner color=white, outer color = red] (\x+0.15,\yb+0.23) circle (0.06);\shade[inner color=white, outer color = red] (\x+0.35,\yb+0.23) circle (0.06);}              
              \node[] at(2.9,3.0) {\scriptsize (a) $J_M\approx -5.2,~\Delta\approx -0.05$};         
		\end{tikzpicture} 
\end{document}
